# Supplementary material for: DETECT: Deep Trajectory Clustering for Mobility-Behavior Analysis
Source: arXiv:2003.01351 source file (2020-03-03)
Supplement: Supplementary file 1 [file appendix.tex]

\clearpage
\appendix
\section*{Appendix}
\setcounter{figure}{0}
\setcounter{table}{0}
\makeatletter 
\renewcommand{\thefigure}{A\@arabic\c@figure}
\renewcommand{\thetable}{A\@arabic\c@table}
\makeatother
\section{Stay point detection algorithm: Fast-SPD}
\label{app:spd}
Algorithm~\ref{alg:fastspd} presents the pseudo code of Fast-SPD. We also compare the speeds of SPD and Fast-SPD. Figure~\ref{fig:spdtime} depicts the computation time of stay points with respect to the length of the trajectory.
We observe that Fast-SPD has similar efficiency on short trajectories($\sim$1k points) but performed much faster as the length of trajectory increases. 
The reason is that more spatial buffers are used in Fast-SPD as the length of trajectory grows. 
Specifically, Fast-SPD requires less time than SPD for refining the candidate points to verify and extract a stay point. 
\textbf{TODOMIGNXUAN, in the figure change trajectory length to trajectory cardinality}
\begin{figure}[htbp]
 \centering
% include the figure here
\includegraphics[width=0.6\columnwidth]{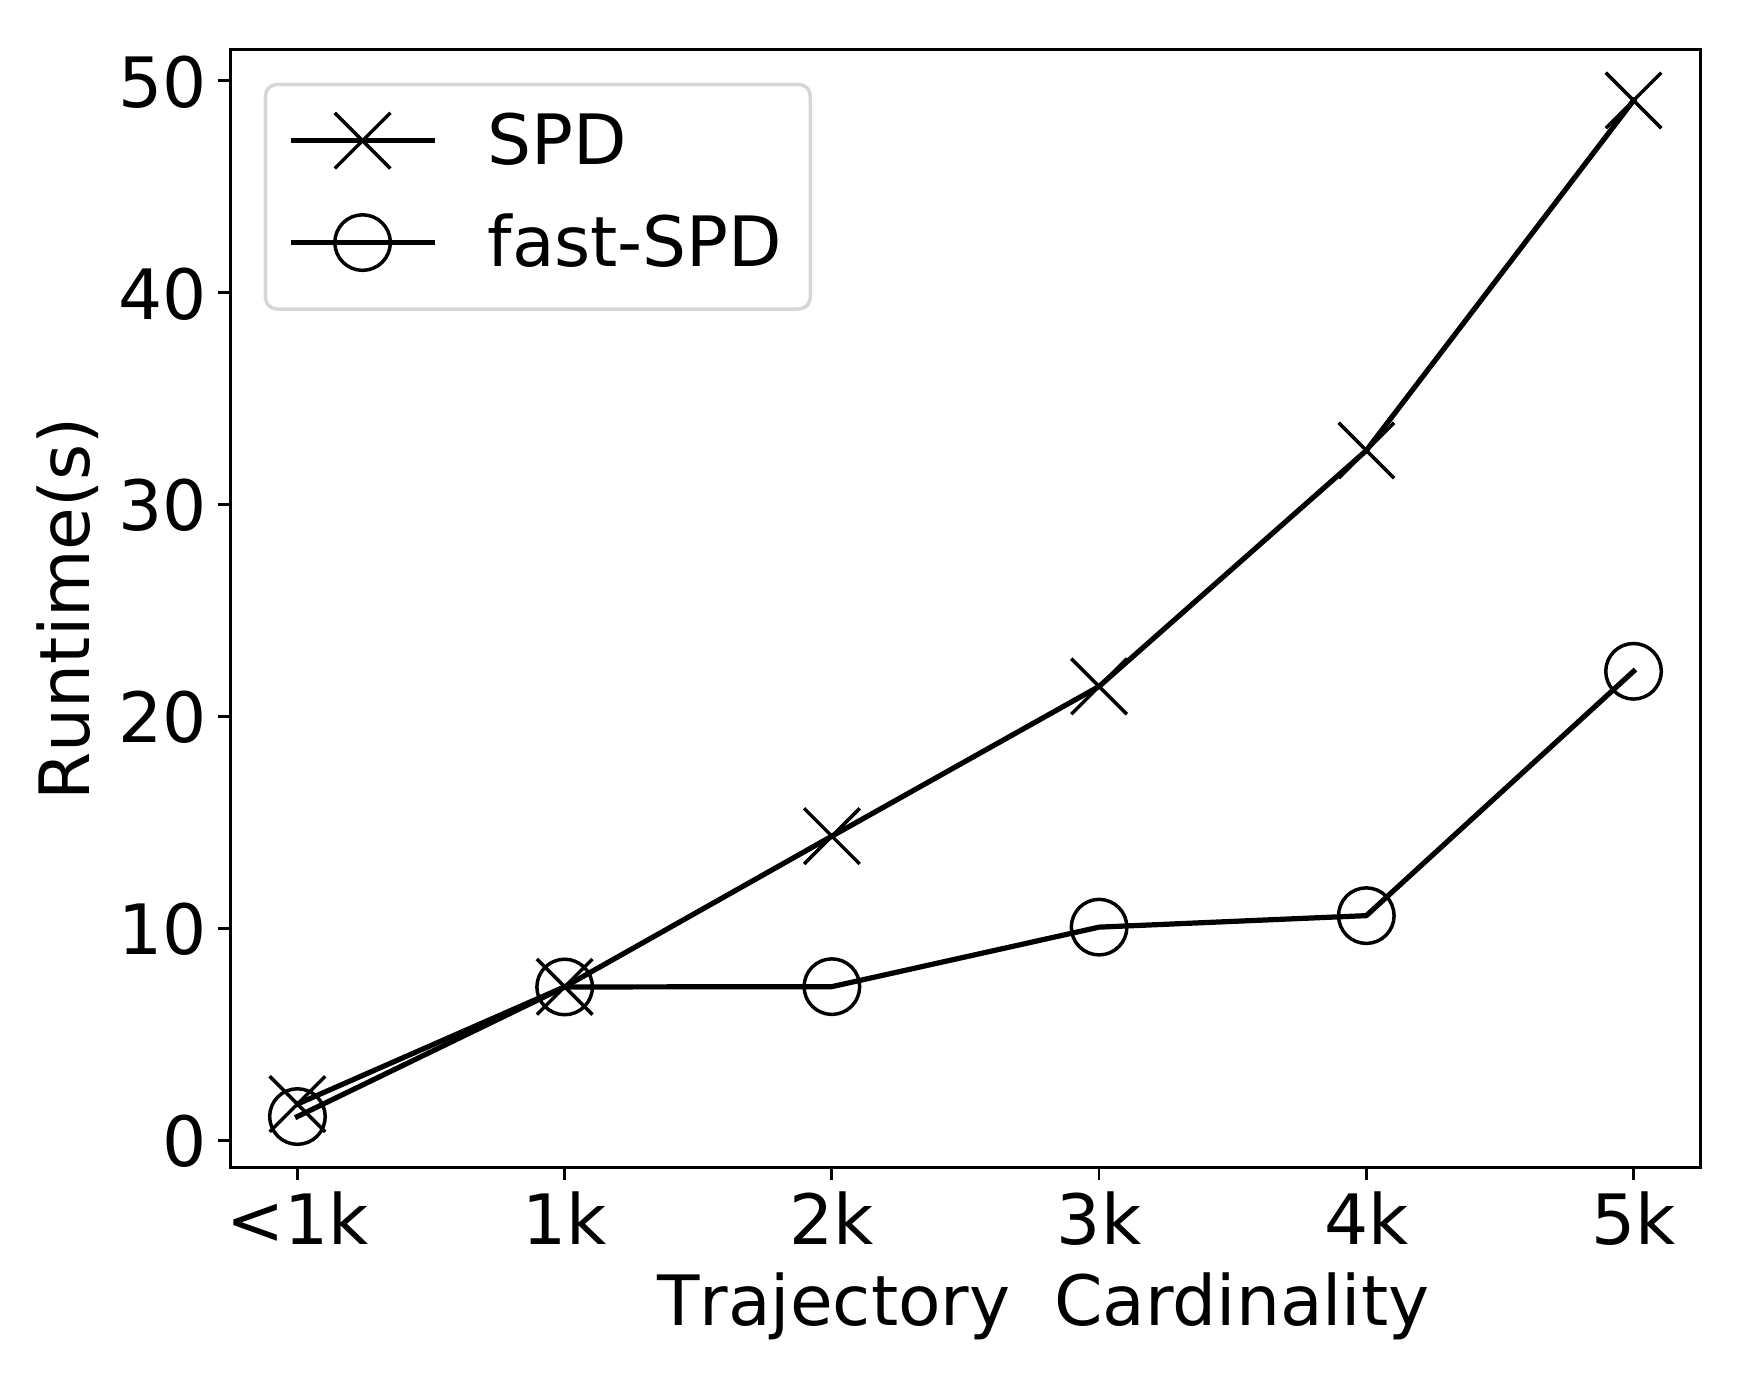}
%\fbox{\rule[-.5cm]{0cm}{2cm} \rule[-.5cm]{2cm}{0cm}}
\caption{Speed comparison between Fast-SPD and SPD}
\label{fig:spdtime}
\end{figure}
